# Supplementary material for: Optimal Control for Wind Turbine Wake Mixing on Floating Platforms
Source: arXiv:2210.17347 source file (2023-03-27)
Supplement: Supplementary file 1 [file appendix.tex]

%!TEX root=../main.tex
